# Supplementary material for: Multipartite entanglement generation and contextuality tests using non-destructive three-qubit parity measurements
Source: arXiv:1902.08842 ancillary file (2019-02-23)
Supplement: Supplementary file 1 [file Supplemental_Material.pdf]

# Supplementary Information for
# Multipartite entanglement generation and contextuality tests using non-destructive three-qubit parity measurements

S.B. van Dam, J. Cramer, T.H. Taminiau, and R. Hanson
*QuTech, Delft University of Technology, 2628 CJ Delft, The Netherlands and*
*Kavli Institute of Nanoscience, Delft University of Technology, 2628 CJ Delft, The Netherlands*

## EXPERIMENTAL SETUP AND MEASUREMENT SEQUENCE

### Experimental setup

We use a naturally occurring NV centre in a chemical-vapour-deposition grown type IIa diamond (Element Six) with a $\langle 111 \rangle$ crystal orientation. The diamond has a natural abundance of carbon isotopes ($\approx 1.1\%$). The samples are kept at a temperature of 4 K in a closed-cycle cryostat (Montana Instruments), in a custom-built confocal microscope. We use a fiber-coupled acousto-optic modulator (Gooche & Housego) for the resonant-excitation (red, 637 nm) laser used for NV electron spin initialisation. Apart from this change the setup is as described in Refs. [1–3].

### Electron-controlled nuclear spin gates

A magnetic field of 415 Gauss is applied approximately along the N-V axis. Table S1 lists the parameters for the nuclear spins 1, 2, and 3 in these conditions, as well as the parameters used for the electron-controlled nuclear gates.

TABLE S1. **Parameters for nuclear qubits and electron-controlled nuclear gates.** The coupling of the carbon nuclear spin qubits to the NV electron spin is characterised by a parallel ($A_\parallel$) and perpendicular ($A_\perp$) hyperfine component, that are parametrised by dynamical decoupling spectroscopy [4]. This results in two relevant nuclear spin precession frequencies: $\omega_0$, when the electron spin state is $m_s = 0$, and $\omega_1$, when the electron spin state is $m_s = -1$. The uncertainty in the measured precession frequencies is around 50 Hz. The change in precession axes for $\omega_0$ and $\omega_1$ is exploited to create electron-controlled nuclear gates [5]. The electron spin is flipped at resonances occurring for half interpulse delays of $\tau \approx k\pi/(2\omega_0 + A_\parallel)$, for integer $k$ [5]. The nuclear spin state is conditionally rotated over a $\pi/2$ angle for $N$ electron spin flips, leading to a total gate time of $2N\tau$.

| | Qubit 1 | Qubit 2 | Qubit 3 |
|---|---|---|---|
| $A_\parallel/(2\pi)$ (kHz) | -372 | -31 | 27 |
| $A_\perp/(2\pi)$ (kHz) | 81 | 29 | 29 |
| $\omega_0/(2\pi)$ (kHz) | 444.1 | 443.9 | 443.7 |
| $\omega_1/(2\pi)$ (kHz) | 820.7 | 476.3 | 417.1 |
| $\tau$ (µs) | 11.469 | 4.884 | 6.402 |
| $N$ | 36 | 44 | 32 |
| gate time (µs) | 826 | 430 | 410 |

The electron-controlled nuclear spin gates are performed by repeated flipping of the electron spin (Fig. S1, top). The gates deviate from a controlled-not (CNOT) gate by a $\pi/2$ rotation along $z$ on the electron, and a $\pi/2$ rotation along $x$ on the nuclear spin (Fig. S1, bottom). We compensate for the rotation on the electron spin in the $\pi/2$ pulse on the electron spin that follows that nuclear spin gate: the rotation axis of this gate depends on the number of nuclear spin gates performed. The $\pi/2$ rotation on the nuclear spin along $x$ is undone by performing the inverse of the unitary operations forming the electron-controlled nuclear gates after the electron readout (Fig 1c).

### measurement sequence

The full circuit diagram describing the measurement sequence for GHZ state generation is shown in Fig. S2. It indicates which unnecessary gates are removed when compiling the sequence. The measurement sequences used for

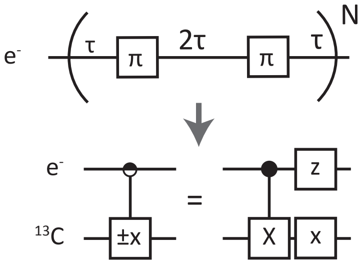


FIG. S1. **Electron-controlled nuclear spin rotation.** The electron-controlled nuclear spin rotation is performed by flipping the electron with an inter-pulse delay $2\tau$. The resulting rotation is equal to a CNOT gate, with an additional $\pi/2$ rotation on the electron spin along $z$ and a $\pi/2$ rotation on the nuclear spin along $x$. In this figure $\pi$ rotations are indicated with capital letters, and small letters indicate $\pi/2$ rotations

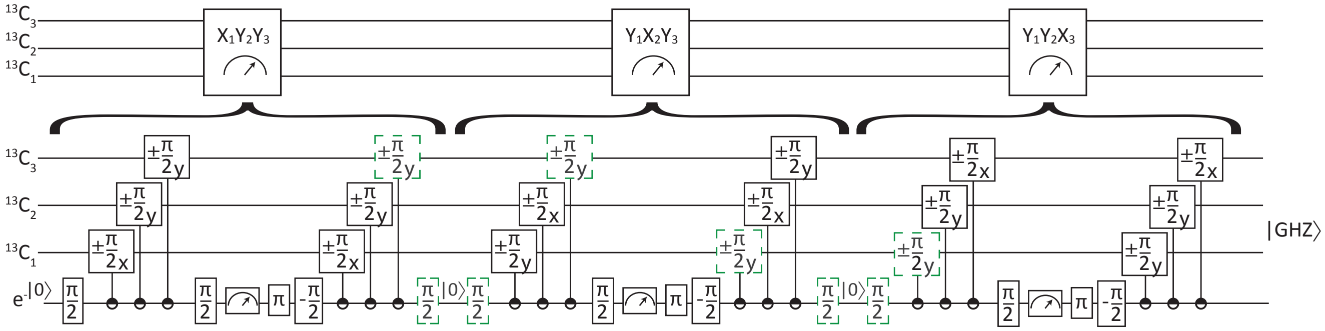


FIG. S2. **Circuit diagram describing the experimental sequence for GHZ state generation.** The sequence shown here incorporates a phase-echoed readout (Fig. 1e). After the GHZ state generation, an additional readout is performed to probe the overlap with a GHZ state. For the single-shot contextuality test (Fig. 3) the three-qubit parity measurement $\sigma_{x,1}\sigma_{x,2}\sigma_{x,3}$ follows. The sequences to test the noncontextuality inequality (Fig. 4) are similar. The elements in green dashed lines are left out when compiling the sequence to minimise gate-induced disturbances. The duration of the electron spin readout is 100 µs. To allow for internal communication time in the setup, the total time between the last $\pi/2$-pulse before the readout, and the spin-echo $\pi$-pulse is 120 µs. To complete the nuclear phase echo, the same wait time is implemented after the $\pi$-pulse, and before the next $\pi/2$-pulse.

the contextuality tests (Figs. 3 and 4) are analogous. Before each measurement run a verification of the NV charge state and that it is on-resonance with the lasers is performed (see, e.g., [1]).

## READOUT CHARACTERISATION

### Electron spin readout

We use the electron spin states $m_s = 0$ and $m_s = -1$ as qubit states. Assuming that both dark states $m_s = +1$ and $m_s = -1$ have the same readout characteristics, we can use both for the readout characterisation (indicated by $m_s = \pm1$). We characterise the electron readout using a maximum likelihood estimation on raw data obtained from two repeated readouts, after initialisation in $m_s = 0$ and $m_s = \pm1$ consecutively.

The model describing these consecutive readouts is in Fig. S3. We denote the probabilities to record "$m_s = 0$" (indicated with subscript $b$ for bright), or "$m_s = \pm1$" (indicated with subscript $d$ for dark) in the consecutive readouts as $p_{0,ij}$ (initial spin state $m_s = 0$), and $p_{1,ij}$ (initial spin state $m_s = \pm1$), with $i \in b, d$ the outcome for the first readout, and $j \in b, d$ the outcome for the second readout. Following the schematic in Fig. S3, we find that the corresponding

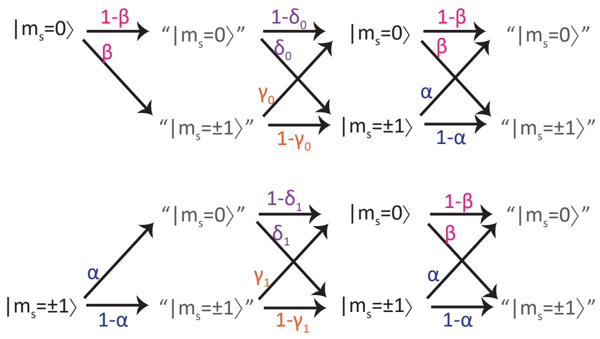


FIG. S3. **Schematic used to model and characterise the readout of the electron spin state.**

probabilities are given by:

$$\begin{aligned}
p_{0,bb} &= (1-\beta)((1-\delta_0)(1-\beta)+\delta_0\alpha); \\
p_{0,bd} &= (1-\beta)((1-\delta_0)\beta+\delta_0(1-\alpha)); \\
p_{0,db} &= \beta(\gamma_0(1-\beta)+(1-\gamma_0)\alpha); \\
p_{0,dd} &= \beta((1-\gamma_0)(1-\alpha)+\gamma_0\beta); \\
p_{1,bb} &= \alpha((1-\delta_1)(1-\beta)+\delta_1\alpha); \\
p_{1,bd} &= \alpha(\delta_1(1-\alpha)+(1-\delta_1)\beta); \\
p_{1,db} &= (1-\alpha)((1-\gamma_1)\alpha+\gamma_1(1-\beta)); \\
p_{1,dd} &= (1-\alpha)((1-\gamma_1)(1-\alpha)+\gamma_1\beta),
\end{aligned} \tag{S1}$$

where $\alpha$, $\beta$, $\gamma_{0,1}$ and $\delta_{0,1}$ are as defined in Fig. S3.

We assume an initialisation probability of $p_{init,0} = 0.998(2)$ for $m_s = 0$ and $p_{init,1} = 0.995(5)$ for $m_s = \pm 1$ [6]. This is taken into account in the probabilities for consecutive readout outcomes for a spin state *intended to be initialised* in $m_s = 0$ ($p_{init,0,ij}$) and in $m_s = \pm 1$ ($p_{init,1,ij}$).

$$\begin{aligned}
p_{init,0,ij} &= p_{init,0}p_{0,ij} + (1-p_{init,0})p_{1,ij} \\
p_{init,1,ij} &= p_{init,1}p_{1,ij} + (1-p_{init,1}) * p_{0,ij}
\end{aligned} \tag{S2}$$

We perform two repeated measurements on a spin state initialised in $m_s = 0$ (5000 repetitions) and $m_s = \pm 1$ (5000 repetitions), leading to $n_{k,ij}$ events per outcome, with $k \in 0,1$ and $i,j \in b,d$. The likelihood function for the corresponding probabilities is [7]:

$$\mathcal{L}(p_{k,ij}) = \frac{n!}{\prod_{k,i,j} n_{k,ij}!} \prod_{k,i,j} p_{init,k,ij}^{n_{k,ij}}, \tag{S3}$$

where $n = \sum_{k,i,j} n_{k,ij}$ is the total number of measurement repetitions. We obtain the values of $\alpha$, $\beta$, $\gamma_0$, $\gamma_1$, $\delta_0$, $\delta_1$ that maximise the likelihood. They are listed in Table S2, and shown in Fig. 1a.

We find confidence intervals for each parameter individually, by finding the value for which the likelihood drops to $1/e$ of its maximum value. We average the upper and lower bounds of the confidence intervals. Additionally, we use the extrema of the confidence intervals in the electron spin initialisation fidelities in the maximum likelihood estimation to find the parameters corresponding to these extreme values. The reported confidence interval in Table S2 and Fig. 1a is the maximum from both methods.

### Nuclear three-qubit parity measurement

To characterise the three-qubit parity measurement on the nuclear spins, we perform three consecutive parity measurements on an initially maximally mixed state. The state is therefore initially equally distributed over the two parity subspaces that we read out: $\langle XXX \rangle = +1$ and $\langle XXX \rangle = -1$. The schematic in Fig. S4 shows the parameters

TABLE S2. **Electron spin readout parameters.** The table lists the parameters of the model in Fig. S3, characterising the electron spin readout extracted using a maximimum likelihood estimation on data from repeated electron spin readouts. These parameters correspond to those in Fig. 1a.

| electron spin readout parameter | estimated value |
|---|---|
| $\alpha$ | $0.007^{+0.003}_{-0.005}$ |
| $\beta$ | $0.050^{+0.002}_{-0.003}$ |
| $\gamma_0$ | $0.05^{+0.02}_{-0.01}$ |
| $\gamma_1$ | $0.000^{+0.001}_{-0.000}$ |
| $\delta_0$ | $0.01^{+0.004}_{-0.004}$ |
| $\delta_1$ | $0.14^{+0.12}_{-0.05}$ |

that determine the probabilities for the readout outcomes of three consecutive measurements with readout outcomes $i$, $j$, and $m$ $(i, j, m \in b, d)$, parameterised by $p_{ijm}$. The resulting probabilities are presented in Eq. (S4). Note that in this method each measurement block is treated independently; it is assumed that there are no correlated errors or coherences between the measurements.

A maximum likelihood estimation from raw data is performed analogously to the procedure as described above for the electron readout. This results in the parameters listed in Table S3, and shown in Fig. 1b.

$$\begin{aligned}
p_{bbb} =&0.5(1-\beta)\Big((1-\delta_0)(1-\beta)\big((1-\delta_0)(1-\beta)+\delta_0\alpha\big)+\delta_0\alpha\big((1-\delta_1)(1-\beta)+\delta_1\alpha\big)\Big)+\\
&0.5\alpha\Big((1-\delta_1)(1-\beta)\big((1-\delta_0)(1-\beta)+(\delta_0\alpha)\big)+\delta_1\alpha\big((1-\delta_1)(1-\beta)+\delta_1\alpha\big)\Big)\\
p_{bbd} =&0.5(1-\beta)\Big((1-\delta_0)(1-\beta)\big((1-\delta_0)\beta+\delta_0(1-\alpha)\big)+\delta_0\alpha\big((1-\delta_1)\beta+\delta_1(1-\alpha)\big)\Big)+\\
&0.5\alpha\Big((1-\delta_1)(1-\beta)\big((1-\delta_0)\beta+\delta_0(1-\alpha)\big)+\delta_1\alpha\big((1-\delta_1)\beta+\delta_1(1-\alpha)\big)\Big)\\
p_{bdb} =&0.5(1-\beta)\Big(\delta_0(1-\alpha)\big((1-\gamma_1)\alpha+\gamma_1(1-\beta)\big)+(1-\delta_0)\beta\big((1-\gamma_0)\alpha+\gamma_0(1-\beta)\big)\Big)+\\
&0.5\alpha\Big(\delta_1(1-\alpha)\big((1-\gamma_1)\alpha+\gamma_1(1-\beta)\big)+(1-\delta_1)\beta\big((1-\gamma_0)\alpha+\gamma_0(1-\beta)\big)\Big)\\
p_{bdd} =&0.5(1-\beta)\Big(\delta_0(1-\alpha)\big((1-\gamma_1)(1-\alpha)+\gamma_1\beta\big)+(1-\delta_0)\beta\big((1-\gamma_0)(1-\alpha)+\gamma_0\beta\big)\Big)+\\
&0.5\alpha\Big(\delta_1(1-\alpha)\big((1-\gamma_1)(1-\alpha)+\gamma_1\beta\big)+(1-\delta_1)\beta\big((1-\gamma_0)(1-\alpha)+\gamma_0\beta\big)\Big)\\
p_{dbb} =&0.5\beta\Big((1-\gamma_0)\alpha\big((1-\delta_1)(1-\beta)+\delta_1\alpha\big)+\gamma_0(1-\beta)\big((1-\delta_0)(1-\beta)+\delta_0\alpha\big)\Big)+\\
&0.5(1-\alpha)\Big((1-\gamma_1)\alpha\big((1-\delta_1)(1-\beta)+\delta_1\alpha\big)+\gamma_1(1-\beta)\big((1-\delta_0)(1-\beta)+\delta_0\alpha\big)\Big)\\
p_{dbd} =&0.5\beta\Big((1-\gamma_0)\alpha\big((1-\delta_1)\beta+\delta_1(1-\alpha)\big)+\gamma_0(1-\beta)\big((1-\delta_0)\beta+\delta_0(1-\alpha)\big)\Big)+\\
&0.5(1-\alpha)\Big((1-\gamma_1)\alpha\big((1-\delta_1)\beta+\delta_1(1-\alpha)\big)+\gamma_1(1-\beta)\big((1-\delta_0)\beta+\delta_0(1-\alpha)\big)\Big)\\
p_{ddb} =&0.5\beta\Big((1-\gamma_0)(1-\alpha)\big(\gamma_1(1-\beta)+(1-\gamma_1)(\alpha)\big)+\gamma_0\beta\big(\gamma_0(1-\beta)+(1-\gamma_0)(\alpha)\big)\Big)+\\
&0.5(1-\alpha)\Big((1-\gamma_1)(1-\alpha)\big(\gamma_1(1-\beta)+(1-\gamma_1)(\alpha)\big)+\gamma_1\beta\big(\gamma_0(1-\beta)+(1-\gamma_0)(\alpha)\big)\Big)\\
p_{ddd} =&0.5\beta\Big((1-\gamma_0)(1-\alpha)\big((1-\gamma_1)(1-\alpha)+(\gamma_1\beta)\big)+\gamma_0\beta\big((1-\gamma_0)(1-\alpha)+(\gamma_0\beta)\big)\Big)+\\
&0.5(1-\alpha)\Big((1-\gamma_1)(1-\alpha)\big((1-\gamma_1)(1-\alpha)+(\gamma_1\beta)\big)+\gamma_1\beta\big((1-\gamma_0)(1-\alpha)+(\gamma_0\beta)\big)\Big)
\end{aligned} \tag{S4}$$

## MEASUREMENT COMPATIBILITY

In a noncontextuality inequality like the one in Eq. 3 and tested in Fig. 4, it is assumed that the measurements within each context are compatible. However, for realistic parity measurements that are subject to experimental

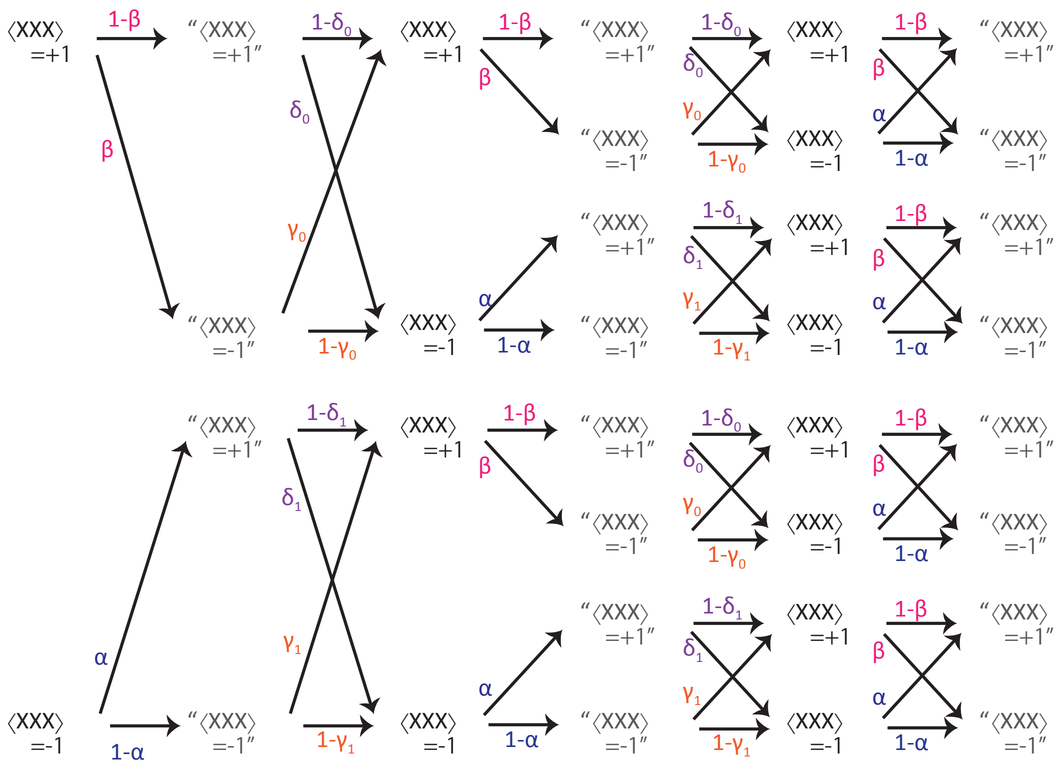

FIG. S4. **Schematic used to model and characterise the nuclear three-qubit parity measurement.**

TABLE S3. **Three qubit parity readout parameters.** The table lists the parameters obtained for the model in Fig. S4, characterising the three-qubit parity readout extracted using a maximimum likelihood estimation on data from repeated three-qubit parity measurements. These parameters correspond to those in Fig. 1b.

| three-qubit parity readout parameter | estimated value |
|---|---|
| $\alpha$ | $0.056^{+0.004}_{-0.004}$ |
| $\beta$ | $0.092^{+0.006}_{-0.006}$ |
| $\gamma_0$ | $0.05^{+0.03}_{-0.03}$ |
| $\gamma_1$ | $0.034^{+0.006}_{-0.005}$ |
| $\delta_0$ | $0.062^{+0.007}_{-0.007}$ |
| $\delta_1$ | $0.000^{+0.027}_{-0.000}$ |

imperfections, the compatibility is imperfect. We characterise the compatibility of the measurements appearing in Eq. 3 by consecutively applying measurements A-B-A. We show the probability to find the same outcome for measurement A in the last round as in the first round in Figs. S5 and S6. Figure S5 contains the results for phase branched measurements (Fig. 1d), and Fig. S6 for the phase echoed measurements (Fig. 1e). The average probability to find the same outcome for A twice is 84% and 82% for the two types of measurements consecutively.

We observe an asymmetry in the measurement compatibility between outcome "+1" and outcome "-1", that is the result of the asymmetry in the assignment fidelity for the electron readout (Fig. 1). We further see that measurements that contain more electron-controlled nuclear spin gates (i.e. the three-qubit parity measurements) have reduced compatibility compared to measurements with single electron-controlled nuclear spin gates.

In the characterisation we include measurements of the type A-A-A, i.e. where the same measurement is performed three times (gray bars in Figs. S5 and S6). The probability to measure the same outcome for the first and third of these measurements in these cases is comparable to the situations where A-B-A is measured for any measurement B with the same number of electron-controlled gates as A. This indicates that the incompatibility is the result of measurement disturbances that act similarly for each measurement, and thus is not likely exploited by a 'classical demon' to reproduce a contextual classical model. However, we emphasize that due to the consecutive nature of the measurements, such a 'demonic' behaviour cannot be formally ruled out. Measurement compatibility is therefore

TABLE S4. **GHZ state generation results.** The table lists outcome probabilities ($p_{outcome}$) and fidelities with the corresponding GHZ state ($F_{GHZ}$) for the data shown in Fig. 2 (phase-branched) and Fig. S7 (phase-echoed). The measurement is repeated 10000 times for each final readout along one of the seven non-zero components of the ideal GHZ states (70000 repetitions in total). The parity measurements $p_1$, $p_2$, and $p_3$ and their outcomes $P_1$, $P_2$, and $P_3$ are described in Eq. 1.

| outcome $P_1$ | outcome $P_2$ | outcome $P_3$ | GHZ state | phase-branched | | phase-echoed | |
|---|---|---|---|---|---|---|---|
| | | | | $p_{outcome}$ | $F_{GHZ}$ | $p_{outcome}$ | $F_{GHZ}$ |
| +1 | +1 | +1 | $\frac{1}{\sqrt{2}}(\|000\rangle - \|111\rangle)$ | 0.104 | 0.68(1) | 0.106 | 0.63(1) |
| +1 | +1 | −1 | $\frac{1}{\sqrt{2}}(\|001\rangle + \|110\rangle)$ | 0.117 | 0.64(1) | 0.117 | 0.62(1) |
| +1 | −1 | +1 | $\frac{1}{\sqrt{2}}(\|010\rangle + \|101\rangle)$ | 0.118 | 0.66(1) | 0.115 | 0.62(1) |
| +1 | −1 | −1 | $\frac{1}{\sqrt{2}}(\|011\rangle - \|100\rangle)$ | 0.134 | 0.62(1) | 0.134 | 0.58(1) |
| −1 | +1 | +1 | $\frac{1}{\sqrt{2}}(\|011\rangle + \|100\rangle)$ | 0.115 | 0.65(1) | 0.113 | 0.63(1) |
| −1 | +1 | −1 | $\frac{1}{\sqrt{2}}(\|010\rangle - \|101\rangle)$ | 0.130 | 0.64(1) | 0.130 | 0.60(1) |
| −1 | −1 | +1 | $\frac{1}{\sqrt{2}}(\|001\rangle - \|110\rangle)$ | 0.126 | 0.65(1) | 0.124 | 0.60(1) |
| −1 | −1 | −1 | $\frac{1}{\sqrt{2}}(\|000\rangle + \|111\rangle)$ | 0.157 | 0.57(1) | 0.161 | 0.54(1) |

needed as additional assumption in the test of the noncontextuality inequality.

## GHZ STATE GENERATION - ADDITIONAL DATA AND RESULTS

Table S4 lists the fidelity and probability of creation of each of the eight GHZ states through the application of three consecutive parity measurements. Figure S7 shows the measurement results corresponding to the generation of a GHZ state using three consecutive parity measurements that employ an electron $\pi$-pulse during the readout to echo the nuclear spin phases (as described in Fig. 1e).

## CONTROL SEQUENCE SIMULATION

Simulations of the control sequences in Figs. 2, 3 and 4, and Fig. S7 are performed by density matrix evolution simulations. We present the parameters that were used as input to the simulations in Table S5.

During electron readout, an outcome corresponding to an electron spin flip is assumed to result in carbon dephasing, modelled as a dephasing channel. The parameters for the electron readout are obtained using the model in Fig. S3, in which the dark state consists of both $m_s = -1$ and $m_s = +1$. We thus assume that the readout parameters are the same for each of the dark states. A spin flip from $m_s = 0$ during readout is simulated to have equal probability to go to the $m_s = -1$ and $m_s = +1$ states. The electron readout parameters used in the simulation are listed in Table S5.

Nuclear spin gate errors are modelled as resulting in a mixed nuclear spin state:

$$\rho_{new} = (2F_g - 1)\hat{G}\rho_{old}\hat{G}^\dagger + (2 - 2F_g)Id, \tag{S5}$$

where $\rho_{old(new)}$ are the old and new density matriced representing the nuclear spin state, $\hat{G}$ is the ideal nuclear spin gate operator, $Id$ is the identity matrix representing the maximally mixed state, and we define $F_g$ as the gate fidelity.

The gate fidelity is independently determined from characterisation measurements in which the nuclear spin is initialised in $|X\rangle$ and then read out along $|X\rangle$. The final result is first corrected for the electron spin readout infidelity. Then, as both initialisation and readout employ a single electron-controlled nuclear spin gate, the full infidelity in the final state is attributed to the application of two nuclear spin gates: in this analysis we assume that the errors in each gate are independent. We average the gate fidelities found for the three employed nuclear spins, to obtain a single value for the nuclear spin gate fidelity, listed in Table S5. Any separate influence of dephasing of the nuclear spins is neglected in the simulations.

TABLE S5. **Parameters used in simulations of the control sequence.** The parameters for the electron spin readout correspond to the model described in Fig. S3. Values used in the simulations deviate from those in Table S2, as averages over several measurements are used to get a best estimate for the parameters during the experiment, that are subject to setup drifts. The nuclear gate fidelity in the simulations is the same for each nuclear spin state; the simulation parameter is determined from the average of individual nuclear gate fidelities. The number of significant digits does not represent the level of certainty in the experimentally determined gate fidelity. The calibration error in the nuclear spin precession frequency is estimated from a calibration of the spin echo pulse during the readout, and in the simulations only effective during the electron readout. The error is accounted for in the precession frequency when the electron is in the spin state $m_s = -1$ ($\omega_1$) for all qubits. For qubit 1, that has larger $A_\parallel$ (see Table S1), the error is additionally applied to the precession frequency when the electron is in $m_s = 0$ ($\omega_0$).

| | |
|---|---|
| assignment fidelity $m_s = 0$ $(1-\beta)$ | 0.94765 |
| assignment fidelity $m_s = -1$ $(1-\alpha)$ | 0.9877 |
| $\gamma_0$ | 0.05 |
| $\gamma_1$ | 0.00 |
| $\delta_0$ | 0.00 |
| $\delta_1$ | 0.1 |
| nuclear gate fidelity | 0.988233 |
| calibration error $\omega_1$ (qubit 1,2,3), $\omega_0$ (qubit 1) | 0.014% |

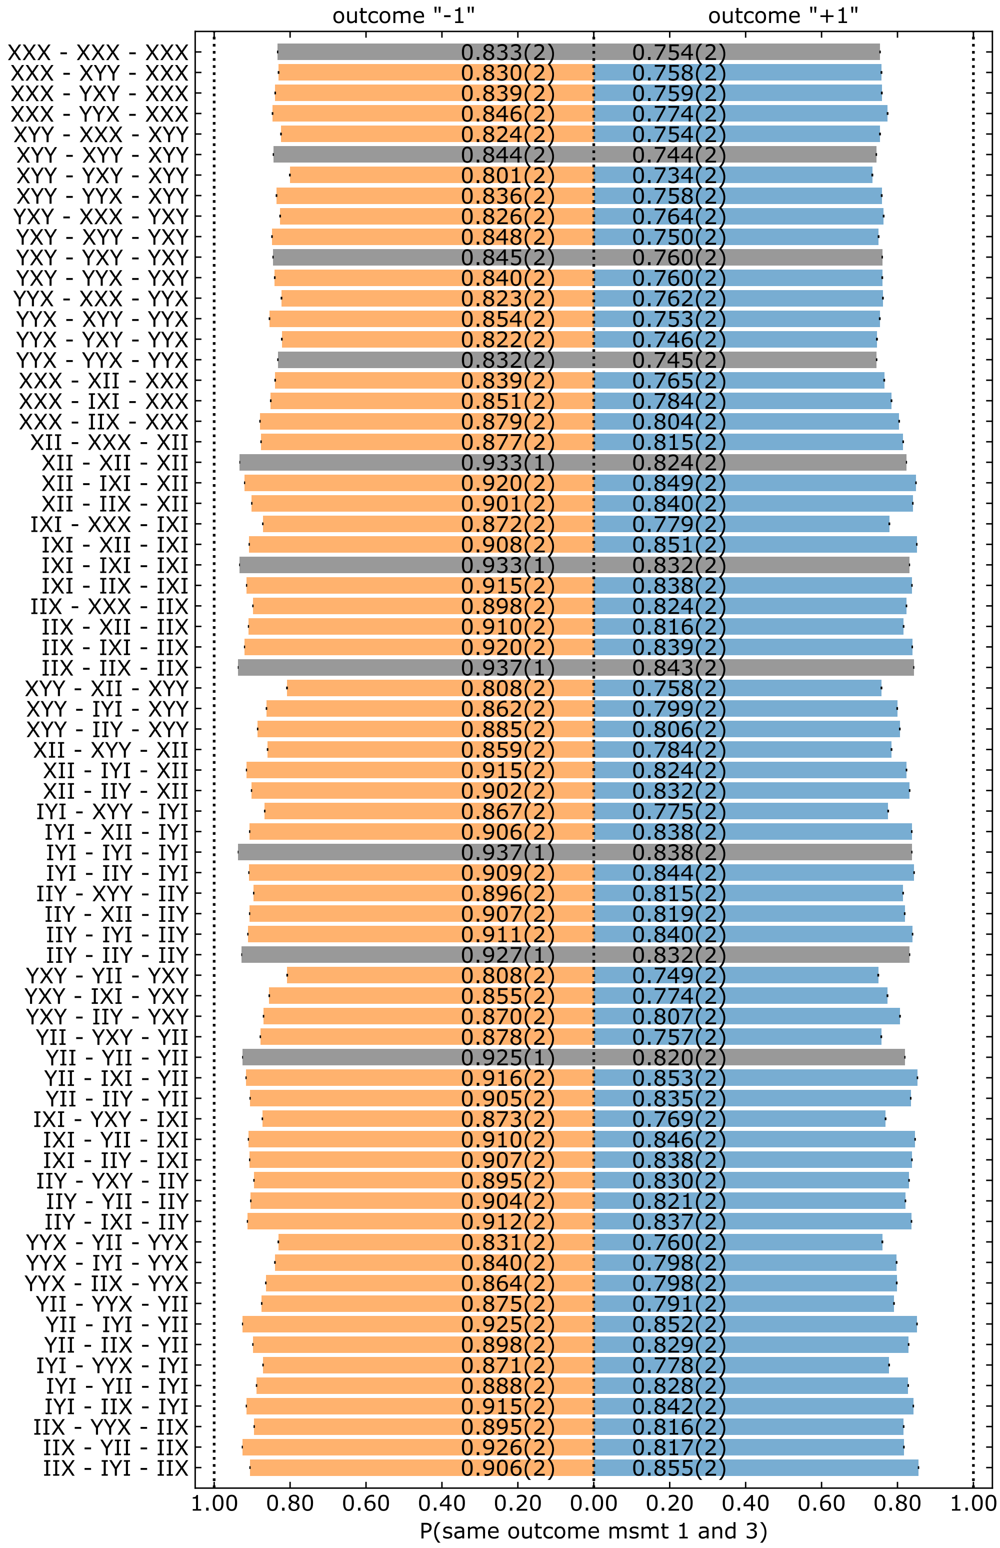


FIG. S5. **Measurement compatibility of phase-branched measurements.** The figure shows the probability to get the same readout outcome for measurement A twice when measuring A-B-A. The probability to find outcome $-1(+1)$ in the third measurement after measuring $-1(+1)$ in the first measurement are shown on the left hand side (right hand side). Gray bars correspond to cases where the middle measurement is the same as the first and third (measuring A-A-A). The average probability to get the same outcome for measurement A twice is 84%.

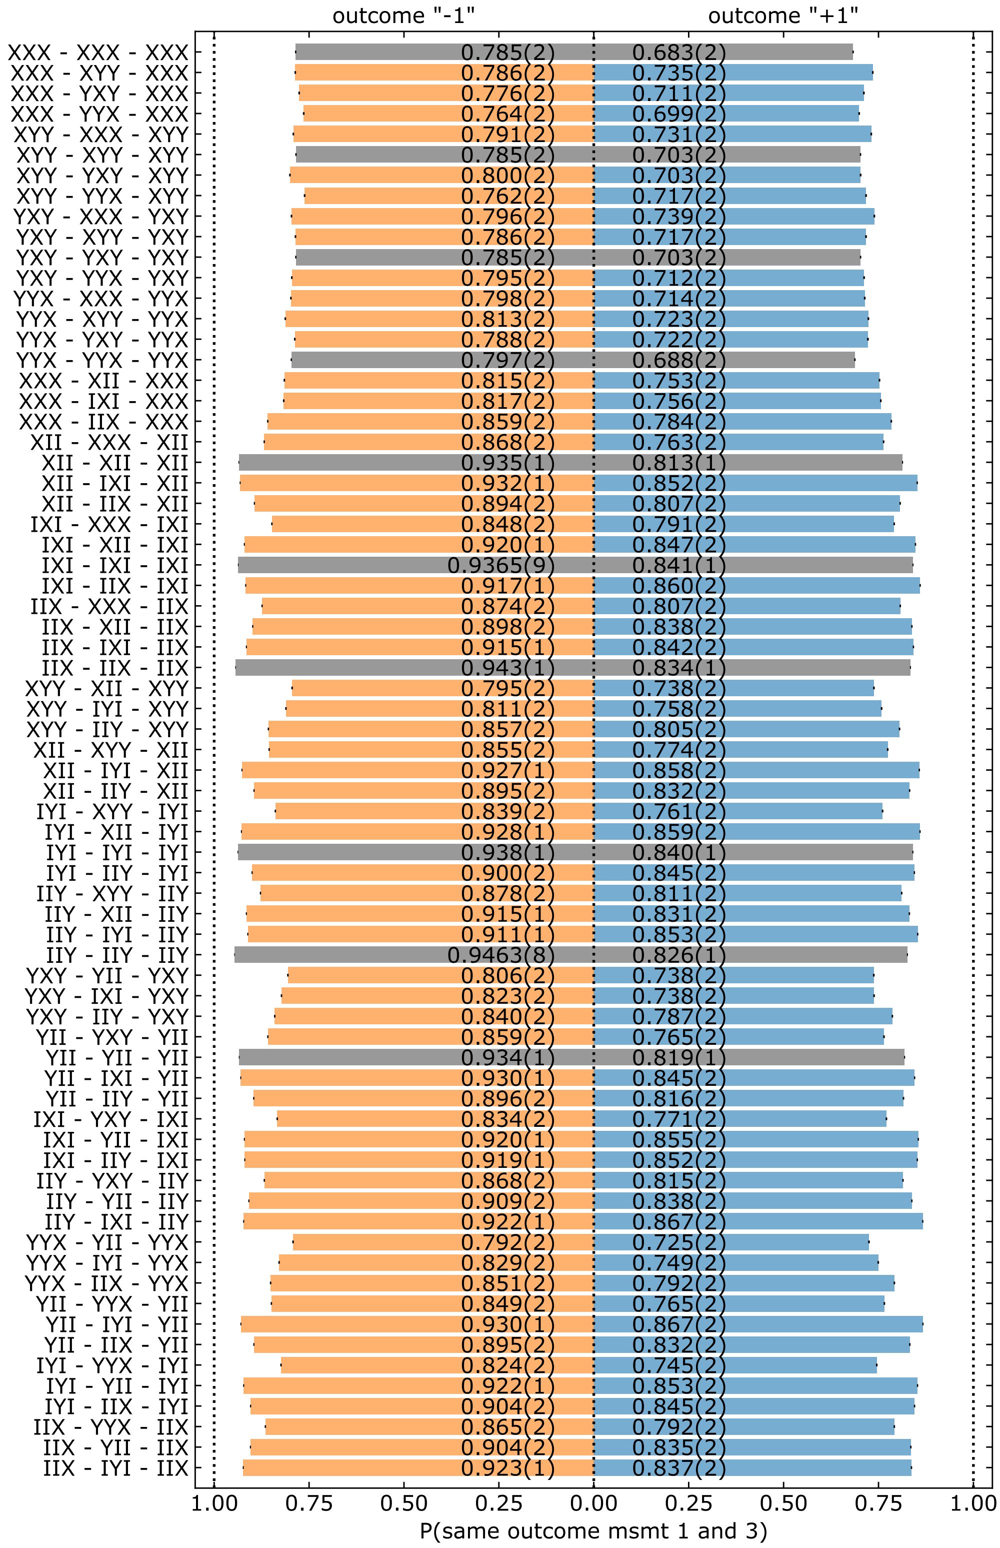


FIG. S6. **Measurement compatibility of phase-echoed measurements.** The figure shows the probability to get the same readout outcome for measurement A twice when measuring A-B-A. The probability to find outcome $-1(+1)$ in the third measurement after measuring $-1(+1)$ in the first measurement are shown on the left hand side (right hand side). Gray bars correspond to cases where the middle measurement is the same as the first and third (measuring A-A-A). The average probability to get the same outcome for measurement A twice is 82%.

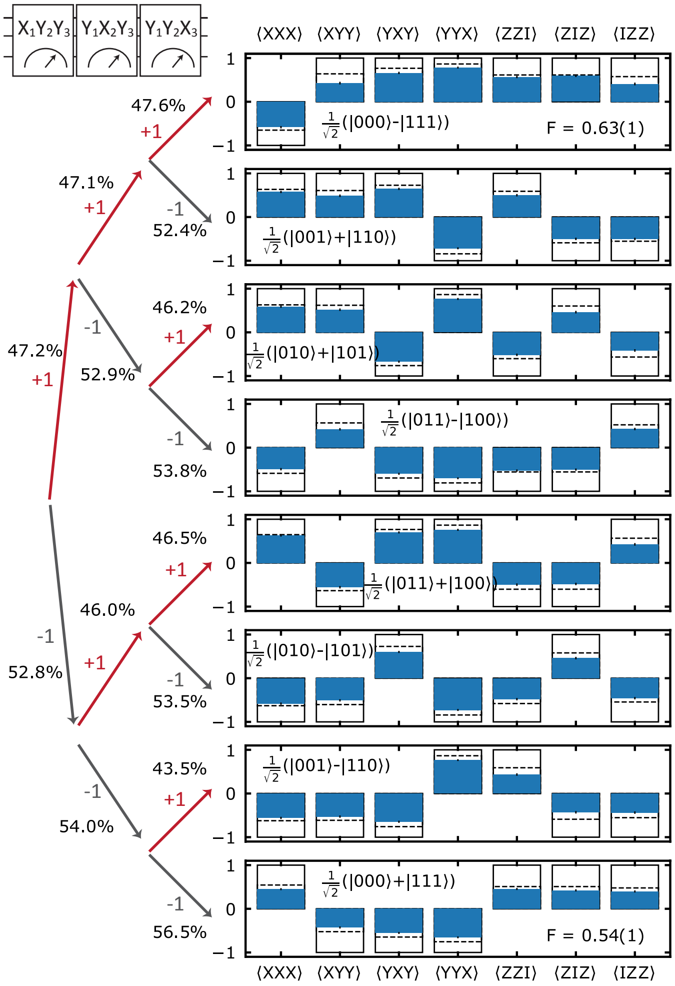


FIG. S7. **Creating a GHZ state by consecutive parity measurements with spin echo.** Conditional on the outcomes of three consecutive parity measurements one out of eight maximally entangled GHZ states is created out of an initially mixed state. The data shown here (blue bars) is obtained using phase-echoed measurements (see Fig. 1e). Black lines indicate the ideal outcome for a GHZ state, and black dashed lines are the outcome of a simulation with independently characterised parameters. To obtain the best estimate for the nuclear state the final readout is corrected for electron spin readout infidelity.

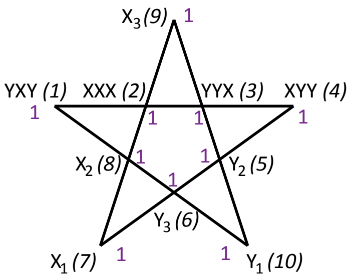


FIG. S8. **Schematic representation of the noncontextuality inequality (Eq. (S6)).** The numbering of the measurements as used in Eq. (S8) is written in parenthesis behind each measurement. A preassigned set of measurement outcomes is depicted that maximizes the winning probability $\beta_{win}$.

## HYPOTHESIS TEST FOR THE NONCONTEXTUALITY INEQUALITY

To perform a hypothesis test on the data (Fig. 4) obtained for the noncontextuality inequality (NCI, Eq. 3), we transform the inequality into a win/lose game [8]. A round of the proposed game is won if the readout outcomes satisfy the following results:

$$\begin{aligned}
&X_1 \times Y_2 \times Y_3 \times XYY_{123} = 1; \\
&Y_1 \times X_2 \times Y_3 \times YXY_{123} = 1; \\
&Y_1 \times Y_2 \times X_3 \times YYX_{123} = 1; \\
&X_1 \times X_2 \times X_3 \times XXX_{123} = 1; \\
&XYY_{123} \times YXY_{123} \times YYX_{123} \times XXX_{123} = -1,
\end{aligned} \tag{S6}$$

where, e.g., $X_1$ represents the outcome of measuring $\sigma_x$ on qubit 1, and $XYY_{123}$ represents the readout outcome for the three-qubit parity measurement $\sigma_{x,1} \otimes \sigma_{y,2} \otimes \sigma_{y,3}$.

Following a noncontextual hidden-variable (NCHV) model and assuming measurement compatibility, the maximum winning probability is $\beta_{win} = 4/5$, as we show below. Following quantum mechanics, a winning probability of 1 can be achieved.

### Maximum winning probability following a NCHV model

We show the maximum bound on the winning probability for a NCHV model following the approach described in Ref. [9]. For a certain distribution $\mu$ over hidden variables $h$, the win probability is given by:

$$\beta_{win} = \int \mathrm{d}\mu(h) \sum_{(i,j,k,l)\in\mathcal{D}} \Pr(\#1 = i, \#2 = j, \#3 = k, \#4 = l, h) \Pr(win|\#1 = i, \#2 = j, \#3 = k, \#4 = l, h), \tag{S7}$$

where $i, j, k, l$ are the four consecutively applied measurements picked from one of the five contexts depicted in Fig. S8:

$$\mathcal{D} = (1, 2, 3, 4), (4, 5, 6, 7), (7, 8, 2, 9), (9, 3, 5, 10), (10, 6, 8, 1). \tag{S8}$$

Since we perform measurements from the five contexts with equal probability, we get:

$$\beta_{win} = \frac{1}{5} \int \mathrm{d}\mu(h) \sum_{(i,j,k,l)\in\mathcal{D}} \Pr(win|\#1 = i, \#2 = j, \#3 = k, \#4 = l, h). \tag{S9}$$

We assume here that the distribution over hidden variables that determines the measurement outcomes is the same in every trial of the experiment, i.e. they are independent and identically distributed (i.i.d) [9]. We now split up the set of contexts in two separate sets:

$$\mathcal{D}_1 = (1, 2, 3, 4). \tag{S10}$$

$$\mathcal{D}_2 = (4, 5, 6, 7), (7, 8, 2, 9), (9, 3, 5, 10), (10, 6, 8, 1). \tag{S11}$$

The win probability for the first set $\mathcal{D}_1$ is maximised for combinations of measurement outcomes with a negative product, whereas for the second set a maximum win probability is achieved with positive-product combinations. We write:

$$\begin{aligned}
\beta_{win} = \frac{1}{5}\int \mathrm{d}\mu(h)\Big\{ &\Pr(win|\#1=1,\#2=2,\#3=3,\#4=4,h) \\
&+ \sum_{(i,j,k,l)\in\mathcal{D}_2} \Pr(win|\#1=i,\#2=j,\#3=k,\#4=l,h)\Big\} \qquad (S12)\\
= \frac{1}{5}\int \mathrm{d}\mu(h)\Big\{ &\Pr(A_1=1,A_2=1,A_3=1,A_4=-1|\#1=1,\#2=2,\#3=3,\#4=4,h) + \textit{neg.comb.} \\
&+ \sum_{(i,j,k,l)\in\mathcal{D}_2} \Big(\Pr(A_i=1,A_j=1,A_k=1,A_l=1|\#1=i,\#2=j,\#3=k,\#4=l,h) + \textit{pos.comb.}\Big)\Big\} \qquad (S13)\\
= \frac{1}{5}\int \mathrm{d}\mu(h)\Big\{ &\Pr(A_1=1|\#1=1,h)\Pr(A_2=1|\#1=1,\#2=2,h)\Pr(A_3=1|\#1=1,\#2=2,\#3=3,h) \\
&\times \Pr(A_4=-1|\#1=1,\#2=2,\#3=3,\#4=4,h) + \textit{neg.comb.} \\
&+ \sum_{(i,j,k,l)\in\mathcal{D}_2} \Big(\Pr(A_i=1|\#1=i,h)\Pr(A_j=1|\#1=i,\#2=j,h)\Pr(A_k=1|\#1=i,\#2=j,\#3=k,h) \\
&\times \Pr(A_l=1|\#1=i,\#2=j,\#3=k,\#4=l,h) + \textit{pos.comb.}\Big)\Big\} \qquad (S14)\\
= \frac{1}{5}\int \mathrm{d}\mu(h)\Big\{ &\Pr(A_1=1|\#1=1,h)\Pr(A_2=1|\#1=2,h)\Pr(A_3=1|\#1=3,h)\Pr(A_4=-1|\#1=4,h) + \textit{neg.comb.} \\
+ \sum_{(i,j,k,l)\in\mathcal{D}_2} &\Big(\Pr(A_i=1|\#1=i,h)\Pr(A_j=1|\#1=j,h)\Pr(A_k=1|\#1=k,h)\Pr(A_l=1|\#1=l,h) + \textit{pos.comb.}\Big)\Big\}. \qquad (S15)
\end{aligned}$$

With *pos.comb.* we indicate all additional combinations of measurement outcomes that have a positive product, and with *neg.comb.* we indicate all those with a negative product. To go from Eq. (S13) to Eq. (S14) we assume causality: measurements performed later in time cannot have an influence on earlier measurements. Going from Eq. (S14) to Eq. (S15) we assume measurement compatibility within each context. This means that we can equate, e.g.:

$$\Pr(A_j=1|\#1=i,\#2=j,h) = \Pr(A_j=1|\#1=j,h). \qquad (S16)$$

Note that the assumption of measurement compatibility can also replace the assumption of causality that we used to go from Eq. (S13) to Eq. (S14).

We aim to find the maximum $\beta_{win}$ for any probability mass $\mathrm{d}\mu(h)$. A maximum is achieved for a deterministic distribution [9], that we can in principle already find from Eq. (S15). We however first continue to simplify the expression in Eq. (S15), expressing each term in probabilities of obtaining outcome +1. We write, e.g.:

$$\Pr(A_4=-1|\#1=4,h) = 1-\Pr(A_4=1|\#1=4,h) =: 1-\Pr(A_4), \qquad (S17)$$

where we introduce the notation $\Pr(A_m)$ as a shorthand for the expression $\Pr(A_m=1|\#1=m,h)$. We write out

explicitly all combinations contained in *neg.comb.* and *pos.comb.*, and simplify the resulting expression, finding:

$$\begin{aligned}\beta_{win} = \frac{1}{5}\int \mathrm{d}\mu(h)\Big\{ & \Pr(A_1)+\Pr(A_2)+\Pr(A_3)+\Pr(A_4)-2\Pr(A_1)\Pr(A_2)-2\Pr(A_1)\Pr(A_3)-2\Pr(A_1)\Pr(A_4)\\ & -2\Pr(A_2)\Pr(A_3)-2\Pr(A_2)\Pr(A_4)-2\Pr(A_3)\Pr(A_4)+4\Pr(A_1)\Pr(A_2)\Pr(A_3)+4\Pr(A_1)\Pr(A_2)\Pr(A_4)\\ & +4\Pr(A_1)\Pr(A_3)\Pr(A_4)+4\Pr(A_2)\Pr(A_3)\Pr(A_4)-8\Pr(A_1)\Pr(A_2)\Pr(A_3)\Pr(A_4)\\ & +\sum_{(i,j,k,l)\in\mathcal{D}_2}\Big(1-\Pr(A_i)-\Pr(A_j)-\Pr(A_k)-\Pr(A_l)+2\Pr(A_i)\Pr(A_j)+2\Pr(A_i)\Pr(A_k)+2\Pr(A_i)\Pr(A_l)\\ & +2\Pr(A_j)\Pr(A_k)+2\Pr(A_j)\Pr(A_l)+2\Pr(A_k)\Pr(A_l)-4\Pr(A_i)\Pr(A_j)\Pr(A_k)-4\Pr(A_i)\Pr(A_j)\Pr(A_l)\\ & -4\Pr(A_i)\Pr(A_k)\Pr(A_l)-4\Pr(A_j)\Pr(A_k)\Pr(A_l)+8\Pr(A_i)\Pr(A_j)\Pr(A_k)\Pr(A_l)\Big)\Big\} \quad \text{(S18)}\\ & \leq \frac{4}{5}. \quad \text{(S19)}\end{aligned}$$

As there are four sets of $(i,j,k,l)\in\mathcal{D}_2$, the constant term, 1, within the sum over $(i,j,k,l)\in\mathcal{D}_2$ in Eq. (S18) results in a total constant term of 4. We take it out of the integral, and can evaluate the remaining terms in the integral, aiming to find the maximum winning probability optimizing over the probability mass $\mathrm{d}\mu(h)$. A maximum is achieved for a deterministic distribution [9]; an example of a distribution that maximises $\beta_{win}$ is shown in Fig. S8. For this distribution (and other optimal distributions) the integral over the probabilities evaluates to 0, and the maximum classical winning probability, following a NCHV model, is found to be $\beta_{win,max} = 4/5$.

## Hypothesis test

Using the maximum winning probability for a NCHV model, we perform a hypothesis test as described in Ref. [8]:

$$p\text{-}value \leq \sum_{i=c}^{n}\binom{n}{i}(\beta_{win,max})^{i}(1-\beta_{win,max})^{(n-i)}, \quad \text{(S20)}$$

where $n$ is the total number of rounds played, and $c$ is the number of wins. The p-value is the maximum probability that a NCHV would have resulted in at least as many wins as the observed data. We assume that the NCHV model does not use memory. For the data presented in Fig. 4, $n = 25000$ and $c = 20477$, resulting in a p-value of $1.21\times10^{-14}$. Assuming measurement compatibility, this is the probability to obtain our data if the experiment is described by a NCHV model.

We note that the assumption of measurement compatibility is unavoidable in state-independent contextuality tests, where due to the consecutive nature of the parity measurements, influences between measurements cannot be excluded by a physical argument (like, e.g., no-signaling). Analysis methods have been designed that include various models of measurement incompatibility [9, 10]; such an analysis is currently not viable for the experimental results presented here.

---


[1] B. Hensen, H. Bernien, A. E. Dréau, A. Reiserer, N. Kalb, M. S. Blok, J. Ruitenberg, R. F. L. Vermeulen, R. N. Schouten, C. Abellán, W. Amaya, V. Pruneri, M. W. Mitchell, M. Markham, D. J. Twitchen, D. Elkouss, S. Wehner, T. H. Taminiau, and R. Hanson, Nature **526**, 682 (2015).

[2] N. Kalb, A. A. Reiserer, P. C. Humphreys, J. J. W. Bakermans, S. J. Kamerling, N. H. Nickerson, S. C. Benjamin, D. J. Twitchen, M. Markham, and R. Hanson, Science **356**, 928 (2017).

[3] P. C. Humphreys, N. Kalb, J. P. J. Morits, R. N. Schouten, R. F. L. Vermeulen, D. J. Twitchen, M. Markham, and R. Hanson, Nature **558**, 268 (2018).

[4] T. H. Taminiau, J. J. T. Wagenaar, T. Van Der Sar, F. Jelezko, V. V. Dobrovitski, and R. Hanson, Phys. Rev. Lett. **109**, 137602 (2012).

[5] T. H. Taminiau, J. Cramer, T. van der Sar, V. V. Dobrovitski, and R. Hanson, Nat. Nanotechnol. **9**, 171 (2014).

[6] L. Robledo, H. Bernien, T. van der Sar, and R. Hanson, New J. Phys. **13**, 025013 (2011).

[7] H. Bernien, B. Hensen, W. Pfaff, G. Koolstra, M. S. Blok, L. Robledo, T. H. Taminiau, M. Markham, D. J. Twitchen, L. Childress, and R. Hanson, Nature **497**, 86 (2013).

[8] D. Elkouss and S. Wehner, npj Quantum Inf. **2**, 16026 (2016).
[9] M. Jerger, Y. Reshitnyk, M. Oppliger, A. Potočnik, M. Mondal, A. Wallraff, K. Goodenough, S. Wehner, K. Juliusson, N. K. Langford, and A. Fedorov, Nat. Commun. **7**, 3 (2016).
[10] O. Gühne, M. Kleinmann, A. Cabello, J.-Å. Larsson, G. Kirchmair, F. Zähringer, R. Gerritsma, and C. F. Roos, Phys. Rev. A **81**, 022121 (2010).
